# Supplementary material for: Equivariance and Invariance Inductive Bias for Learning from Insufficient Data
Source: arXiv:2207.12258 source file (2022-09-06)
Supplement: Supplementary file 1 [file nico_data.tex]

\begin{table*}[t]
\captionsetup{font=footnotesize,labelfont=footnotesize,skip=1pt}
\centering
\caption{Construction of the NICO subset~\cite{he2021towards,wang2021causal} for OOD multi-classification. \textbf{Context} denotes the context class name, while \textbf{Class} represents the object class name. ``Long-Tailed Contexts'' is the training contexts arranged by the sample number order (from more to less) and ``Zero-shot Contexts'' represents the context labels only appear in testing rather than training.
}
\scalebox{0.6}{
    \begin{tabular}{ccccccccccc}
\toprule\toprule
\diagbox{\textbf{Class}}{\textbf{Context}}    & \multicolumn{7}{c}{Long-Tailed Contexts}                                                & \multicolumn{3}{c}{Zero-shot Contexts}     \\ \cmidrule(lr){1-1}\cmidrule(lr){2-8}\cmidrule(lr){9-11}
Dog      & on grass  & in water     & in cage   & eating       & on beach  & lying    & running   & at home      & in street    & on snow     \\ \hline
Cat      & on snow   & at home      & in street & walking      & in river  & in cage  & eating    & in water     & on grass     & on tree     \\ \hline
Bear     & in forest & black        & brown     & eating grass & in water  & lying    & on snow   & on ground    & on tree      & white       \\ \hline
Sheep    & eating    & on road      & walking   & on snow      & on grass  & lying    & in forest & aside people & in water     & at sunset   \\ \hline
Bird     & on ground & in hand      & on branch & flying       & eating    & on grass & standing  & in water     & in cage      & on shoulder \\ \hline
Rat      & at home   & in hole      & in cage   & in forest    & in water  & on grass & eating    & lying        & on snow      & running     \\ \hline
Horse    & on beach  & aside people & running   & lying        & on grass  & on snow  & in forest & at home      & in river     & in street   \\ \hline
Elephant & in zoo    & in circus    & in forest & in river     & eating    & standing & on grass  & in street    & lying        & on snow     \\ \hline
Cow      & in river  & lying        & standing  & eating       & in forest & on grass & on snow   & at home      & aside people & spotted     \\ \hline
Monkey   & sitting   & walking      & in water  & on snow      & in forest & eating   & on grass  & in cage      & on beach     & climbing    \\ \bottomrule\bottomrule
\end{tabular}}
\label{tab:nico}
\end{table*}
