# Supplementary material for: Equivariance and Invariance Inductive Bias for Learning from Insufficient Data
Source: arXiv:2207.12258 source file (2022-09-06)
Supplement: Supplementary file 2 [file additional_tool.tex]

\usepackage{amsmath}
\usepackage{amssymb}
\usepackage{booktabs}
\usepackage{color}
\usepackage{algpseudocode} 
\usepackage{enumitem}

\usepackage{enumitem}
\usepackage{mathrsfs}
\usepackage{amsmath}     
\usepackage{graphicx}
\usepackage{caption}
\usepackage{wrapfig}
\usepackage{enumitem} % for enumerate with left margin
\usepackage{tikz} % for drawing text on images
\usepackage{pifont}
\usepackage{bbm}
\usepackage{makecell}
\usepackage{colortbl}
\usepackage{bbding}

% drawing table
\usepackage{multirow}
\usepackage{booktabs}
\usepackage{bm}
\usepackage{diagbox}    % diagonal box in table
\usepackage[pagebackref,breaklinks,colorlinks]{hyperref}

\definecolor{mygray}{gray}{0.9}

\newlength\savewidth
  
\newcolumntype{x}[1]{>{\centering\arraybackslash}p{#1pt}}
\newcolumntype{y}[1]{>{\raggedright\arraybackslash}p{#1pt}}
\newcolumntype{z}[1]{>{\raggedleft\arraybackslash}p{#1pt}}

\definecolor{ABOVE}{HTML}{FF0000}  %
\definecolor{BELOW}{HTML}{39b54a}  %
