# Supplementary material for: Equivariance and Invariance Inductive Bias for Learning from Insufficient Data
Source: arXiv:2207.12258 source file (2022-09-06)
Supplement: Supplementary file 3 [file fig_ir_cropped.tex]

\begin{wrapfigure}{r}{0.45\textwidth}
\captionsetup{font=footnotesize,labelfont=footnotesize}
\centering
\includegraphics[width=0.95\linewidth]{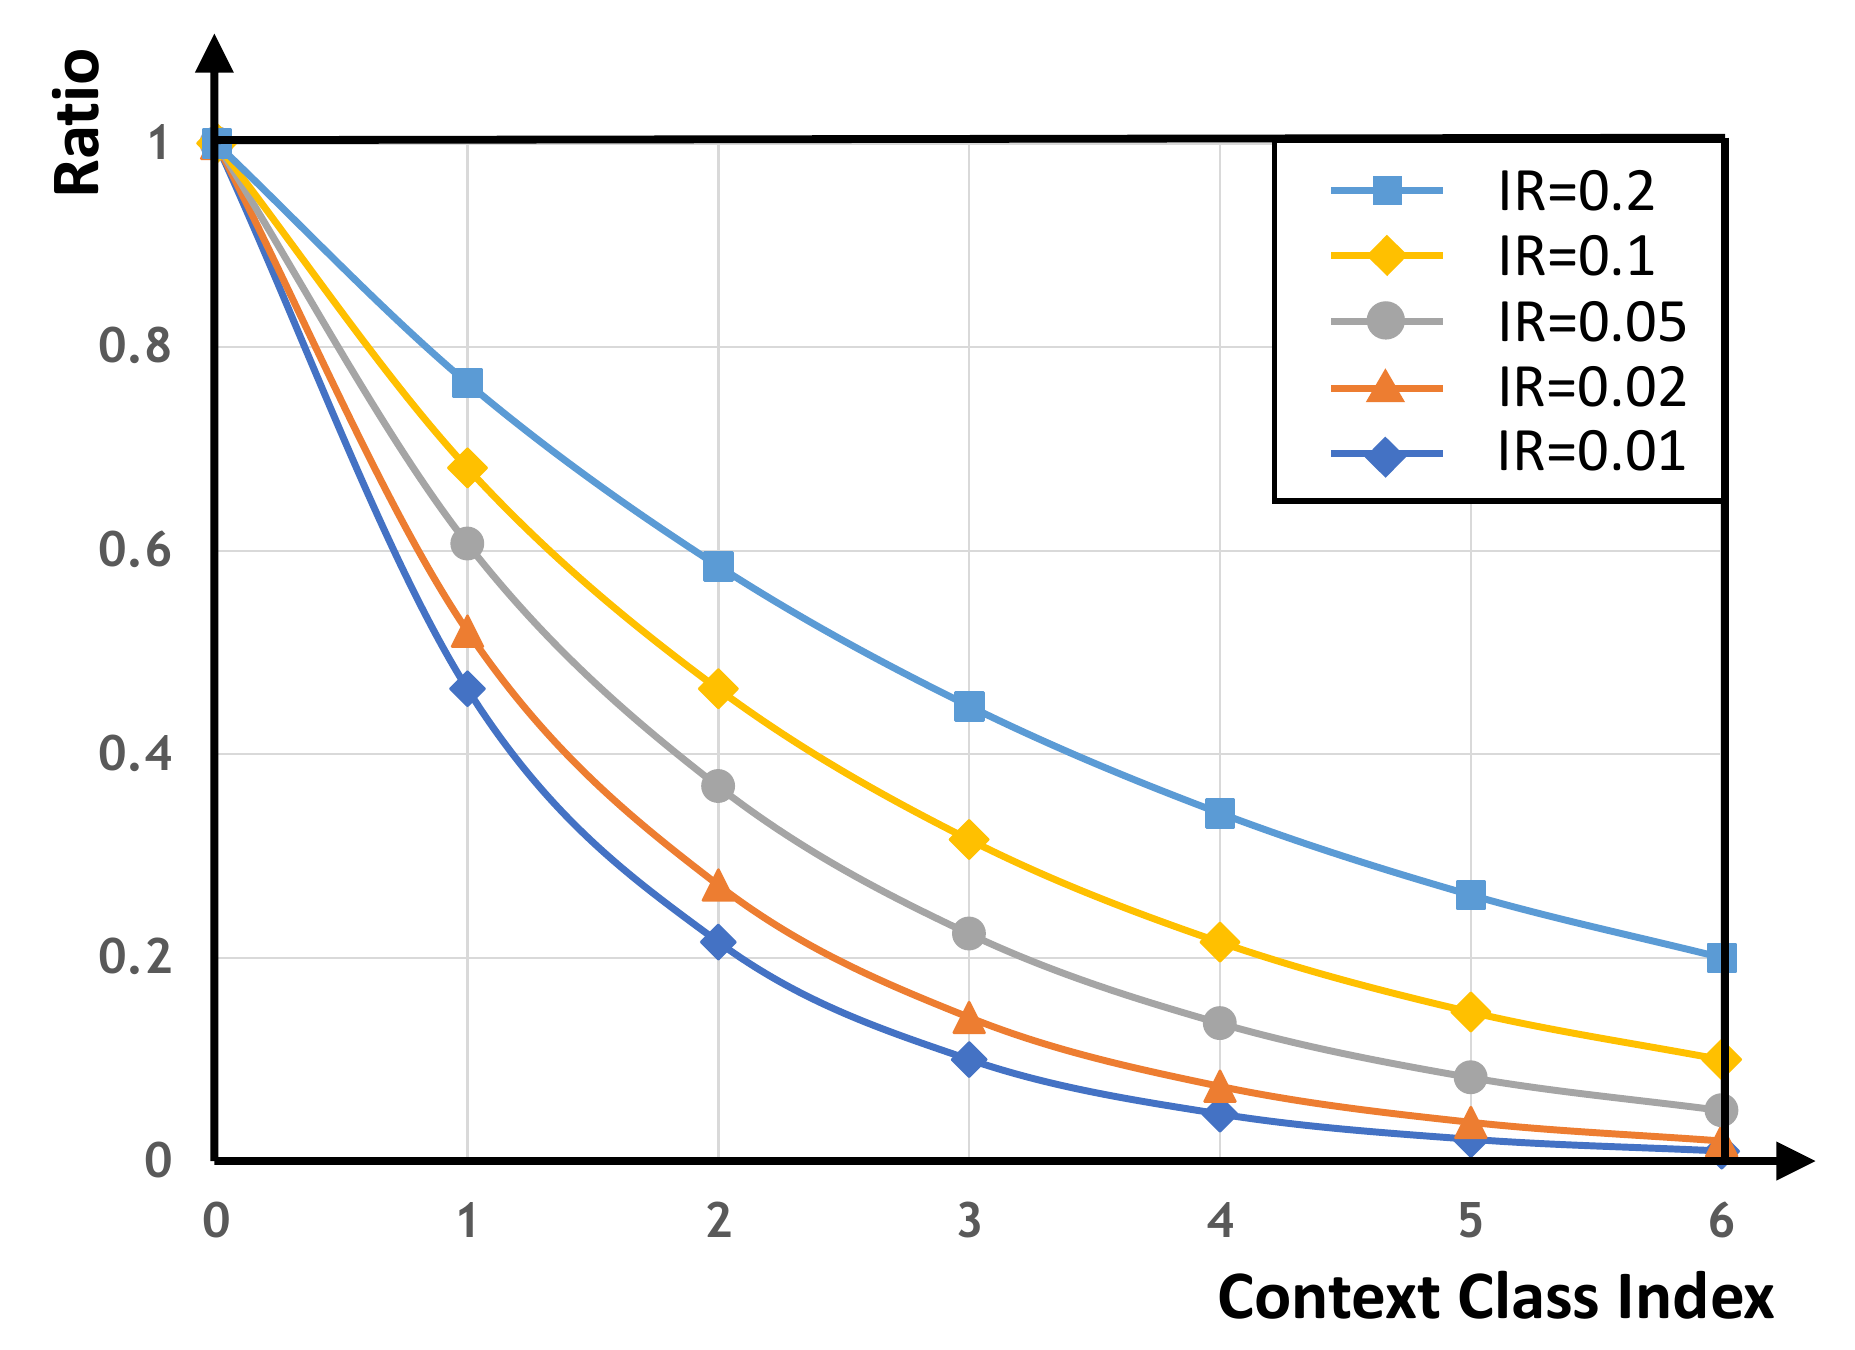}
\caption{Plot of context class index against its corresponding ratio under various imbalance ratio (IR).}
\label{fig:ratio}
\end{wrapfigure}
